# Supplementary material for: Efficient Cross-Shard Transaction Execution in Sharded Blockchains
Source: arXiv:2007.14521 source file (2021-01-29)
Supplement: Supplementary file 1 [file hotstuff.tex]

\section{Hotstuff~\cite{yin2019hotstuff}}
\label{apx:hotstuff}
In this section, we briefly describe the Hotstuff protocol.

Hotstuff is a leader based byzantine fault tolerant SMR protocol that functions in the partial synchrony model. The protocol allows replicas to reach consensus on a single leaf node of the blocktree that constitutes the blockchain. The leaf node represents an entire branch given by the path obtained from the node all the way to the tree root by visiting parent links. The protocol proceeds in a sequence of views numbered with monotonically increasing view numbers. In each view, the replicas run a three phase protocol that begins with the proposal of a tree node (which extends a node that is already a part of the block tree through a parent link) by a leader appointed for that particular view. By the end of the third phase, replicas commit to a node, add it to their local blocktree and execute the commands present in it. If the replicas fail to receive an expected message within a timeout period, or if they have reached consensus on a particular node  they can collectively trigger a view change to replace the leader and  run consensus on a new leaf node in the latter case.The protocol relies heavily on Quorum certificates (QC) or (n-f) distinct signed votes on the same message.

The basic hotstuff protocol can be summarized as follows:

\vspace{1mm}
\noindent
{\bf Prepare phase.} Leader collects (n-f) new view messages from replicas at the beginning of a view. Each new view message contains a \emph{prepareQC} with the highest view number that a replica has encountered.
From among these \emph{prepareQC}’s the leader picks the one with the highest view number \emph{highQC}. The leader extends the tail of node mentinoned in \emph{highQC} with a new leaf node proposal. The new node is proposed(or broadcasted to all replicas) in the form of a prepare message that also carries the \emph{high QC} for justification purposes.

\vspace{1mm}
Replicas check whether the proposed node extends node in \emph{lockedQC} or whether \emph{highQC} has a view number greater than \emph{lockedQC} before accepting the proposal.If found acceptable, the replicas send a prepare vote for the proposal.

\vspace{1mm}
\noindent
{\bf Precommit phase.} The leader combines the prepare votes it receives from (n - f) replicas into a \emph{prepareQC} and broadcasts it in  pre-commit messages. Replicas vote for it with a pre-commit vote that has a signed digest of the proposal.

\vspace{1mm}
\noindent
{\bf Commit phase.}    
The leader combines the pre-commit votes it receives from (n - f) replicas into a \emph{precommitQC} and broadcasts it in  commit messages.Replicas respond with a commit vote and additionally lock themselves on the \emph{precommitQC} by setting their \emph{lockedQC} to the \emph{precommitQC}.

\vspace{1mm}
\noindent
{\bf Decide phase.}
The leader combines the commit votes it receives from (n - f) replicas into a \emph{commitQC} and broadcasts it in  decide messages(signifying a committed decision).Upon receiving the decide message, the replicas execute the commands embedded in the proposal in \emph{commitQC}.The replicas then start the next view by incrementing their view number.

When the leader receives (n-f ) commit votes, it
combines them into a \emph{commitQC}. Once the leader has assembled
a \emph{commitQC}, it sends it in a decide message to all other replicas.
Upon receiving a decide message, a replica considers the proposal
embodied in the \emph{commitQC} a committed decision, and executes the commands in the committed branch.The replica increments viewNumber and starts the next view.

\vspace{1mm}
\noindent
{\bf NextView interrupt.} In all phases, a replica waits for a message
at view \emph{viewNumber} for a timeout period, determined by an auxiliary
\emph{nextView(viewNumber)} utility. If \emph{nextView(viewNumber)}
interrupts waiting, the replica also increments \emph{viewNumber} and
starts the next view.

\begin{fact} (Safety~\cite{yin2019hotstuff})
If w and b are conflicting nodes, then they cannot be both committed, each by a correct replica.
\end{fact}

\begin{fact} (Liveness,~\cite{yin2019hotstuff})
After GST, there exists a bounded time period $T_f$ such
that if all correct replicas remain in view v during $T_f$
and the leader for view v is correct, then a decision is
reached
\end{fact}

To ensure liveness, honest replicas must get a chance to be the leader.This can be achieved with the help of a round robin protocol where there exists a deterministic mapping between the view number and the leader for that view.To ensure that correct replicas remain in a view for atleast $T_f$, one could potentially use an exponential back of mechanism for the the \emph{nextView} utility, that starts a timer at beginning of each view and doubles the timer duration everytime the timer expires.
